# Supplementary material for: Individual low-energy toroidal dipole state in $^{24}$Mg
Source: arXiv:1711.08953 source file (2018-03-29)
Supplement: Supplementary file 1 [file Supplemental_Material.pdf]

# Supplemental Material for: Individual low-energy toroidal dipole state in $^{24}$Mg

V.O. Nesterenko[1], A. Repko [2], J. Kvasil[3], and P.-G. Reinhard[4]
[1] *Laboratory of Theoretical Physics, Joint Institute for Nuclear Research, Dubna, Moscow region, 141980, Russia*
[2] *Department of Nuclear Physics, Institute of Physics SAS, 84511, Bratislava, Slovakia*
[3] *Institute of Particle and Nuclear Physics, Charles University, CZ-18000, Prague 8, Czech Republic and*
[4] *Institut für Theoretische Physik II, Universität Erlangen, D-91058, Erlangen, Germany*
(Dated: January 11, 2018)

## DESCRIPTION OF IV-GDR

In Fig. 1, the isovector giant dipole resonance (IV-GDR) calculated within QRPA with the Skyrme force SLy6 is compared with the experimental data [1, 2]. The photoabsorption $\sigma$ is computed through the isovector energy-weighted strength function [3]. It is smeared by the Lorentz factor with the energy-dependent averaging parameter [3]. Fig. 1 demonstrates a nice agreement of the theory and experiment. This justifies accuracy of our model and relevance of the parametrization SLy6.

## TDR AND CDR STRENGTH FUNCTIONS

In the main text of the paper [4], we basically discuss individual toroidal and compression dipole states in $^{24}$Mg. At the same time, in our previous studies [3, 5–8] and explorations of other groups [9, 10], the toroidal and compression modes were explored through isoscalar toroidal dipole resonance (TDR) and compression dipole resonance (CDR). These two resonances embrace many states and are believed to constitute the low- and high-energy parts of the isoscalar giant dipole resonance (IS-GDR) [10]. In this connection, it is worth to demonstrate the calculated TDR and CDR strengths in $^{24}$Mg and related them with individual toroidal and compression states discussed in the main paper [4].

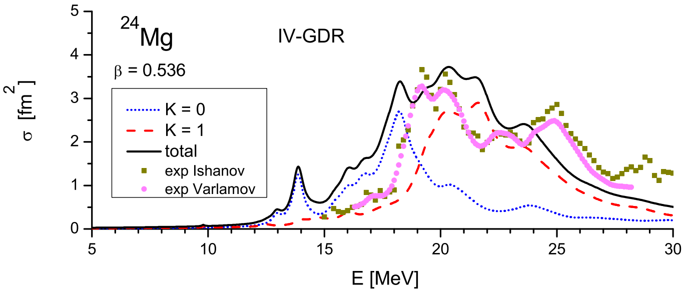


FIG. 1: Photoabsorption in $^{24}$Mg calculated with force SLy6: total (solid black curve), K=0 (blue dotted curve) and K=1 (red dash curve). The results are compared with experimental data [1] (green filed squares) and [2] (purple filled circles).

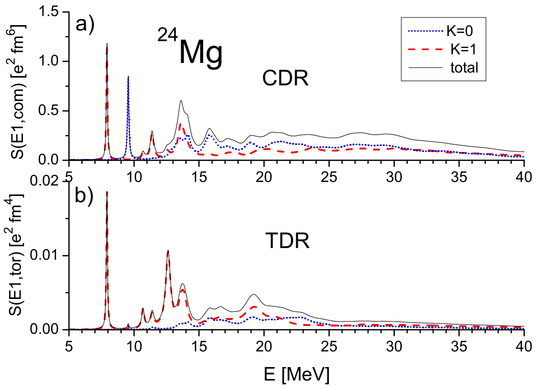


FIG. 2: Isoscalar CDR (a) and TDR (b) strengths in $^{24}$Mg, calculated with the force SLy6. For each case, the total (black solid line), K=0 (blue dotted line) and K=1 (red dash line) strengths are depicted.

The TDR ans CDR strength functions read

$$S\,(E1K,\ \alpha) = \sum_{\nu} B_{\nu}(E1K,\alpha)\,\xi_{\Delta}(E-E_{\nu}) \qquad (1)$$

where $B_{\nu}(E1K,\alpha) = |\ \langle\nu|\ \hat{M}_{\alpha}(\ E1K)\ |0\rangle\ |^2$ is the reduced transition probability between the ground state $|0\rangle$ and QRPA state $|\nu\rangle$, $\hat{M}_{\alpha}(\ E1K)$ is the transition toroidal ($\alpha$ = tor) or compression ($\alpha$=com) dipole operator (see expressions in [4]). Furthermore, $\xi_{\Delta}(E-E_{\nu}) = \Delta(E)/[2\pi[(E-E_{\nu})^2+(\Delta(E))/2)^2]]$ is the Lorentz weight with the energy-dependent averaging parameter $\Delta(E)$ (see details in [3]), $E_{\nu}$ is the energy of the $\nu$-th QRPA dipole state.

Figure 2 demonstrates QRPA strength functions (1) for the isoscalar CDR and TDR. The strengths are obtained with the irrotational density-dependent compression operator (Eq. (4) in [4]) for CDR and the vortical current-dependent toroidal operator (Eq. (2) in [4]) for TDR. Note that the density-dependent CDR operator is customary used as the probe operator in the analysis of IS-GDR [9, 10]. The figure shows that CDR has a broad distribution at 20–40 MeV (which constitutes the main part of the compression mode), some structures at 10–20 MeV, and two well-separated strong peaks at 7.92 MeV (K=1) and 9.56 MeV (K=0). The vortical TDR demonstrates a modest strength at $E > 20$ MeV and similar to CDR structures at 10-20 MeV. So at 10-20 MeV we probably have a mixture of the compression and toroidal

modes. What is remarkable, TDR has the strong low-energy K=1 peak at 7.92 MeV while K=0 peak at 9.56 MeV is fully suppressed. This confirms the previous finding [3, 7, 8] that, in prolate deformed nuclei, the low-energy TDR is dominated by the K=1 strength. Comparing panels a) and b), one may suggest that K=1 state at 7.92 MeV is mainly toroidal (vortical) while K=0 state at 9.56 MeV is basically compressional (irrotational). Occurrence of the toroidal K=1 state in both responses can be explained by a low selectivity of the probe compression external field. The states K=1 state at 7.92 MeV and K=0 at 9.56 MeV are just individual dipole excitations discussed in the main text [4].

## K-ASSIGNMENT OF DIPOLE STATES

Our QRPA calculations with the Skyrme force SLy6 predict the toroidal state as the lowest $I^{\pi}K = 1^{-}1$ excitation at E=7.92 MeV and the compression state as the lowest $1^{-}0$ excitation at E=9.56 MeV [4]. The experimental spectrum below 10 MeV in $^{24}$Mg has three $I^{\pi} = 1^{-}$ states at 7.555, 8.437 and 9.566 MeV [11]. K-assignment of the experimental levels is still ambiguous. The level at 7.555 MeV is often treated as K=0 band head with known $I^{\pi} = 1^{-}, 3^{-}, 5^{-}, 7^{-}$ band members while the level at 8.437 MeV is considered as K=1 band head [12, 13]. However such a treatment of 7.555-MeV level does not agree with Alaga rules [4] and results of recent AMD calculations with Gogny forces, analyzing the triaxiality effect in $^{24}$Mg [14]. AMD results show that the first $1^{-}1$ state should lie below of the first $1^{-}0$ state (in accordance with our finding). AMD calculations also show that triaxially almost does not affect the K=1 band but significantly downshifts the K=0 band. So, one-to-one correspondence of the predicted lowest toroidal and compression dipole states to the experimental dipole levels is not obvious. The toroidal K=1 state can correspond to 7.555-MeV or 8.437-MeV levels. To make the choice unambiguous, we still need a more reliable K-assignment of the experimental dipole levels.


[1] B.S. Ischkhanov, I.M. Kapitonov, E.I. Lileeva, E.V. Shirokov, V.A. Erokhova, M.A. Elkin, A.V. Izotova, Report MSU-INP-2002-27/711 (2002).

[2] V.V. Varlamov, M.E. Stepanov, V.V. Chesnokov, J. Bull. Russ. Acad. Sci. **67**, 724 (2003).

[3] A. Repko, J. Kvasil, V. O. Nesterenko, and P.-G. Reinhard, Eur. Phys. J. A. **53**, 221 (2017).

[4] V.O. Nesterenko, A. Repko, J. Kvasil, and P.-G. Reinhard, main paper.

[5] J. Kvasil, V. O. Nesterenko, W. Kleinig, P.-G. Reinhard, and P. Vesely, Phys. Rev. C**84**, 034303 (2011).

[6] A. Repko, P.-G. Reinhard, V. O. Nesterenko, and J. Kvasil, Phys. Rev. C**87**, 024305 (2013).

[7] J. Kvasil, V. O. Nesterenko, W. Kleinig, and P. - G. Reinhard, Phys. Scr. **89**, 054023 (2014).

[8] V.O. Nesterenko, J. Kvasil, A. Repko, W. Kleinig, P.-G. Reinhard, Phys. Atom. Nucl. **79**, 842 (2016).

[9] M. N. Harakeh and A. van der Woude, *Giant Resonances* (Clarendon Press, Oxford, 2001).

[10] N. Paar, D. Vretenar, E. Kyan, G. Colo, Rep. Prog. Phys. **70**, 691 (2007).

[11] Database [http://www.nndc.bnl.gov].

[12] D. Branford, N. Gardner, and I.F. Wright, Phys. Lett. B, **36**, 456 (1971).

[13] L.K. Fiefield, E.F. Garman, M.J. Hurst, T.J.M. Symons, F. Watt, C.H. Zimmerman, and K.W. Allen, Nucl. Phys. A**322**, 1 (1979).

[14] M. Kimura, R. Yoshida, and M. Isaka, Prog. Theor. Phys., **127**, 287 (2012).
